# Supplementary material for: SpectralGaussians: Semantic, spectral 3D Gaussian splatting for multi-spectral scene representation, visualization and analysis
Source: arXiv:2408.06975 source file (2024-08-13)
Supplement: Supplementary file 1 [file appendix.tex]

\appendix
\section{My Appendix}
% Appendix sections are coded under \verb+\appendix+.

% \verb+\printcredits+ command is used after appendix sections to list 
% author credit taxonomy contribution roles tagged using \verb+\credit+ 
% in frontmatter.
